# Supplementary material for: LayoutVLM: Differentiable Optimization of 3D Layout via Vision-Language Models
Source: arXiv:2412.02193 source file (2025-03-11)
Supplement: Supplementary file 1 [file supp.tex]

% CVPR 2025 Paper Template; see https://github.com/cvpr-org/author-kit

\documentclass[10pt,twocolumn,letterpaper]{article}

\input{inc/inc_packages}
\input{inc/inc_macros}

%%%%%%%%% PAPER TYPE  - PLEASE UPDATE FOR FINAL VERSION
% \usepackage{cvpr}              % To produce the CAMERA-READY version
\usepackage[review]{cvpr}      % To produce the REVIEW version
\usepackage{tabularx}
%\usepackage{cleveref}
% \usepackage[pagenumbers]{cvpr} % To force page numbers, e.g. for an arXiv version

% Import additional packages in the preamble file, before hyperref
\input{preamble}

% It is strongly recommended to use hyperref, especially for the review version.
% hyperref with option pagebackref eases the reviewers' job.
% Please disable hyperref *only* if you encounter grave issues, 
% e.g. with the file validation for the camera-ready version.
%
% If you comment hyperref and then uncomment it, you should delete *.aux before re-running LaTeX.
% (Or just hit 'q' on the first LaTeX run, let it finish, and you should be clear).
\definecolor{cvprblue}{rgb}{0.21,0.49,0.74}
\usepackage[pagebackref,breaklinks,colorlinks,allcolors=cvprblue]{hyperref}

%%%%%%%%% PAPER ID  - PLEASE UPDATE
 % *** Enter the Paper ID here

\usepackage{minted} % For syntax highlighting
\usepackage{mdframed} % For styling frames

% Configure minted options
\setminted{
  fontsize=\scriptsize,
  baselinestretch=.9,
  breaklines=true,
  breakanywhere=true,
  funcnamehighlighting=true,
  tabsize=4,
  obeytabs=false,
  mathescape=false,
  samepage=false,
  showspaces=false,
  showtabs=false,
  texcl=false,
}

% Command to wrap minted output in an mdframed box
% \newcommand{\styledfileinput}[2][text]{% Optional first argument for language
%   \begin{mdframed}[backgroundcolor=gray!10,linewidth=0pt]
%     \inputminted{#1}{#2} % Syntax-highlighted content
%   \end{mdframed}
% }

\begin{document}

% WARNING: do not forget to delete the supplementary pages from your submission 
\input{sec/X_suppl}

\end{document}
